# Supplementary material for: Exploring the apparent violation of the Mott relation in a noncentrosymmetric kagome ferromagnet
Source: arXiv:2512.00173 ancillary file (2025-11-28)
Supplement: Supplementary file 1 [file supp_v7.pdf]

# Supplementary Information: Exploring the apparent violation of the Mott relation in a noncentrosymmetric kagome ferromagnet

Benjamin Kostroun[1,2,3], Tomoya Asaba[4], Sean M. Thomas[5], Eric D. Bauer[5], Sergey Y. Savrasov[6], Filip Ronning[7], and Vsevolod Ivanov[1,2,3]

[1]Department of Physics, Virginia Tech, Blacksburg, VA, 24061 USA
[2]Virginia Tech National Security Institute, Blacksburg, VA, 24060 USA
[3]Virginia Tech Center for Quantum Information Science and Engineering, Blacksburg, VA, 24061 USA
[4]Department of Physics, University of Virginia, Charlottesville, VA, 95616 USA
[5]Materials Physics and Applications Division, Los Alamos National Laboratory, NM, 87545 USA
[6]Department of Physics, University of California, Davis, CA 95616 USA
[7]Institute for Materials Science, Los Alamos National Laboratory, NM, 87545 USA.

## Supplementary Note 1: First-principles LDA+U+J simulations

First principles simulations were performed using the LmtART [S6] code using the LDA+U+J formalism, to understand the effect of exchange coupling on the ferromagnetism in $UCo_{1-x}Ru_xAl$. We scanned the range of Hubbard $U = \{2.04$ eV, 2.72 eV, 3.40 eV, 4.08 eV$\}$, and Hund's $J_H = \{0.0$ eV, 0.2 eV, 0.4 eV, 0.6 eV, 0.8 eV$\}$, defined using the Slater integrals $F^{(2)}$, $F^{(4)}$, $F^{(6)}$ as $J_H = (286F^{(2)} + 195F^{(4)} + 250F^{(6)})/6435$. All calculations were performed on a $6 \times 6 \times 6$ $\boldsymbol{k}$-point grid, with spin-orbit coupling, and spin-restricted double-counting in the fully localized $n^{scf}$ limit was used.

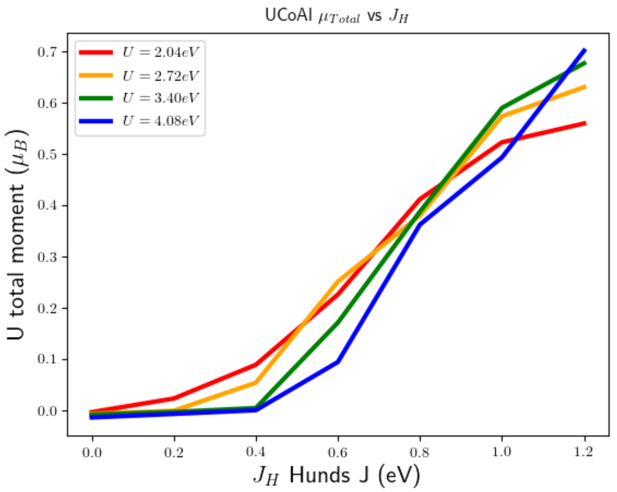


Figure S1: Total magnetic moment on the uranium atom in UCoAl in units of $\mu_B$, as a function of $J_H$.

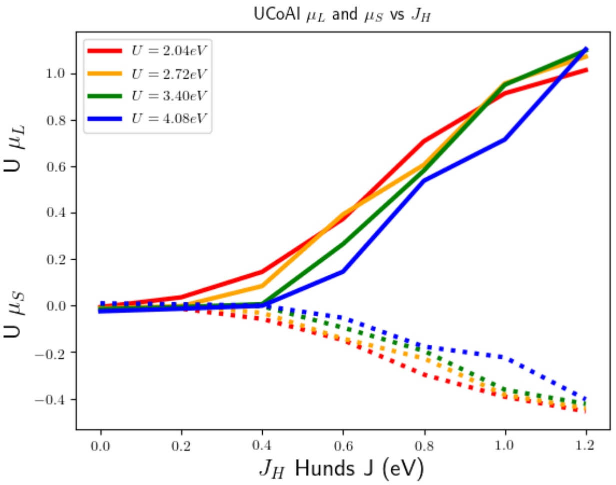


Figure S2: Spin (solid) and orbital (dashed) components of the magnetic moment on the uranium atom in UCoAl in units of $\mu_B$, as a function of $J_H$.

The total magnetic moment on the uranium atom for pure (0% Ru doping) UCoAl is shown in Fig. S1. At the lowest value of Hubbard $U = 2.04$ eV, ferromagnetism appears even at the lowest values of $J_H$. As $U$ increases, a threshold value of $J_H > 0.4$ becomes necessary to induce ferromagnetism. Fig. S2 shows the dependence of spin and orbital components of the magnetic moments. Regardless of the combination of $U$ and $J_H$ values inducing ferromagnetism, the ratio of components is $|\mu_L/\mu_S| \sim 2$, which consistent with the experimentally measured ratio [S4].

We can also model the effect of Ru doping. The unit cell of UCoAl contains 9 atoms, so 1/3 substitution of Co by Ru is possible. Moreover, there is evidence that $UCo_{2/3}Ru_{1/3}Al$ is ordered, with Ru preferentially occupying the $2(c)$ position

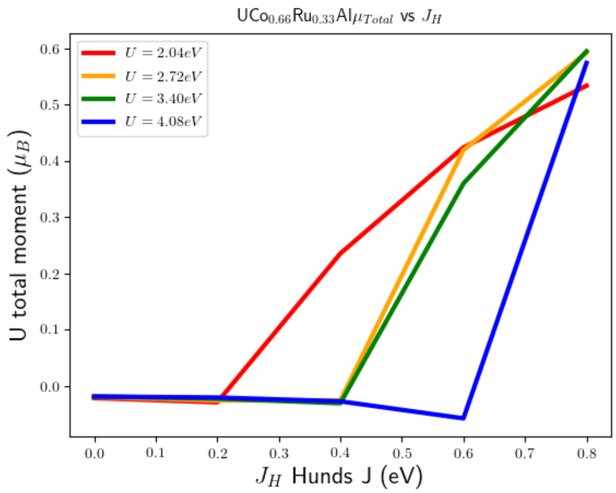


Figure S3: Total magnetic moment on the uranium atom in UCoAl in units of $\mu_B$, as a function of $J_H$.

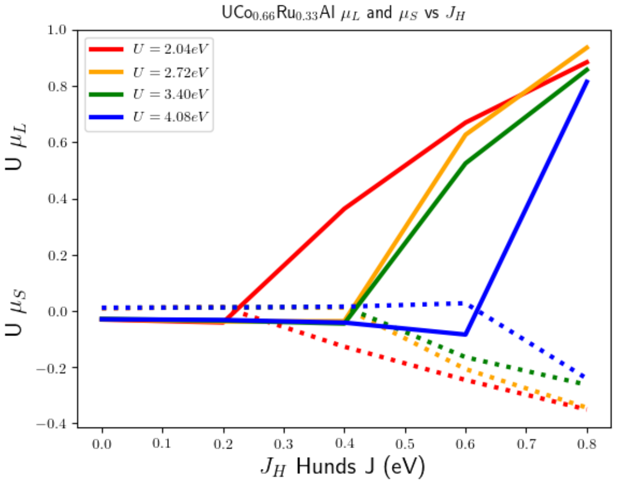


Figure S4: Spin (solid) and orbital (dashed) components of the magnetic moment on the uranium atom in UCoAl in units of $\mu_B$, as a function of $J_H$.

We additionally compute the bandstructure for UCoAl and the projections onto the U$-5f$ and U$-6d$ orbitals. The dense number of bands near the Fermi energy makes it impractical (and likely unenlightening) to create an exact tight-binding model. Instead we construct a minimal model for the Weyl points, with a width of 0.3 eV, and an additional narrow band with a width of 0.2 eV to create a large density of states, emulating the cluster of flat U$-5f$ bands found by first principles calculations (Figure S5).

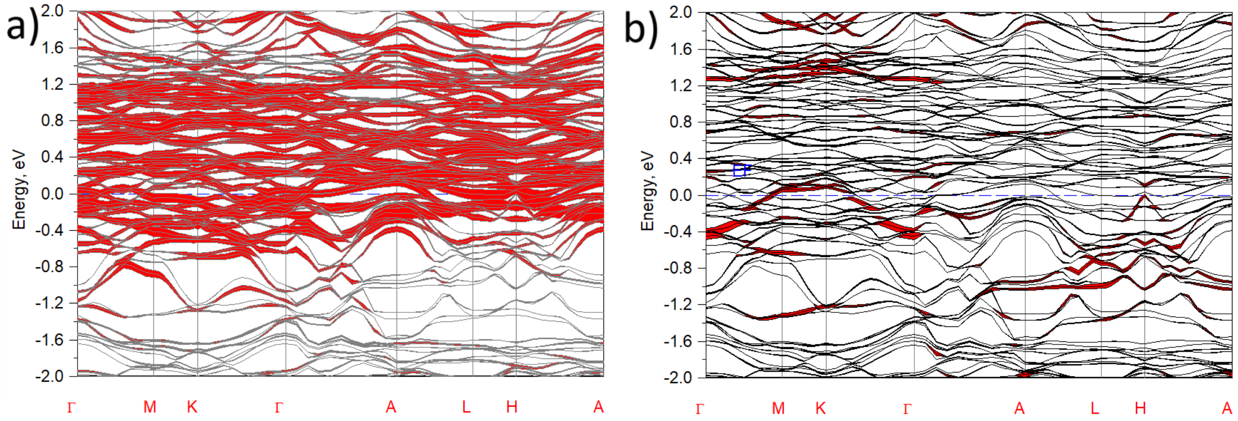


Figure S5: Computed band structure of UCoAl, with projections onto the a) U$-5f$ and b) U$-6d$ orbitals.

We can also compute the density of states, as well as the position of the Fermi level corresponding to the Ruthenium concentrations in the experimental samples (assuming rigid bands). Specifically, we need the values for the concentrations at the mid-points between the sample concentrations: 2.5%, 5%, 10%, 20%, 30%, 50%, 62%, and 70% Ru doping.

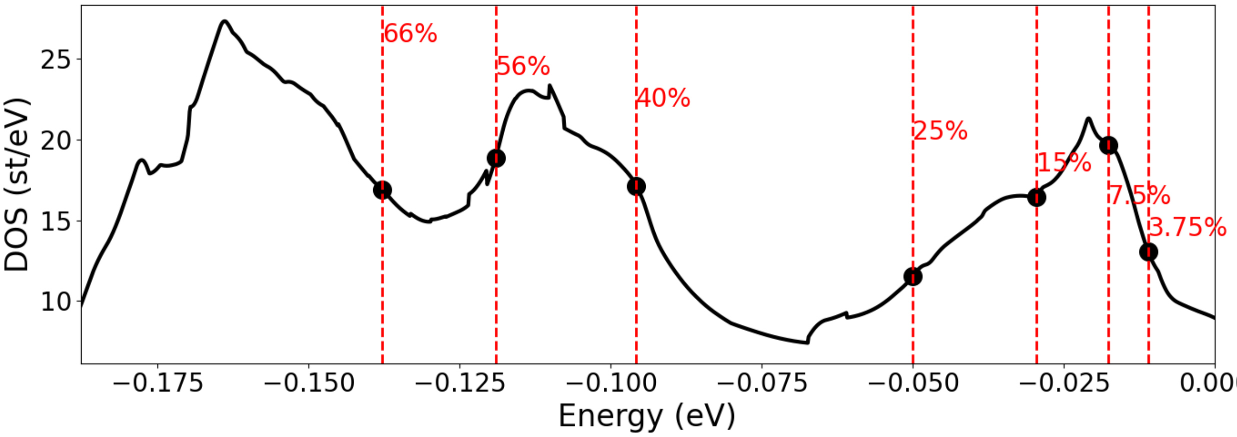


Figure S6: Computed density of states UCoAl, with vertical red lines corresponding to the Fermi level for the corresponding doping, assuming a rigid band shift.

The exact values are provided in the table below:

| Doping | DOS (st./eV) |
|---|---|
| 3.75% | 13.04657605 |
| 7.5% | 19.65274354 |
| 15% | 16.43898005 |
| 25% | 11.52584569 |
| 40% | 17.10509234 |
| 56% | 18.85543956 |
| 66% | 16.91328386 |

To compute the $\alpha_{xy}(n)$ at the dopings $n = (n_{i+1}) + n_i)/2$, as expected from the Mott relation, we use a numerical derivative and the density of states $g(\varepsilon) = \partial n/\partial \varepsilon$ :

$$\alpha_{xy}(n) = \frac{\pi^2 k_B^2 T}{3e}\frac{\partial \sigma_{xy}}{\partial \varepsilon} = \frac{\pi^2 k_B^2 T}{3e}\frac{\partial \sigma_{xy}}{\partial n}\frac{\partial n}{\partial \varepsilon} \approx \frac{\pi^2 k_B^2 T}{3e}\frac{\sigma_{xy}(n_{i+1}) - \sigma_{xy}(n_i)}{n_{i+1} - n_i} g\left(\frac{n_{i+1} + n_i}{2}\right) \tag{1}$$

## Supplementary Note 2: Experimental Details

Single crystals of $UCo_{1-x}Ru_xAl$ were grown by the Czochralski method in a tri-arc furnace with Ru concentrations of $x = 2.5\%, 5\%, 10\%, 20\%, 30\%, 50\%, 60\%, 70\%$. X-ray diffraction confirmed the ZrNiAl-type structure (P-62m, #189). The phase purity and quality of the samples was further confirmed by orienting them and using the X-ray Laue method with a photosensitive detector in a backscattering geometry. The magnetic properties of the samples were in good agreement with prior measurements [S1]. A single setup was used to perform thermoelectric and electronic transport measurements. A 10 kΩ chip resistor was attached to the end of each sample and used to generate a temperature gradient. This was measured with homemade thermocouples made from Fe-doped gold and chromel. The cold sink was provided by a sapphire substrate physically clamped to an oxygen-free copper cold finger. The input heating power was monitored to maintain a linear response with the heating power. Current leads are attached parallel to the sample rather than at a single point of contact to ensure uniform current.

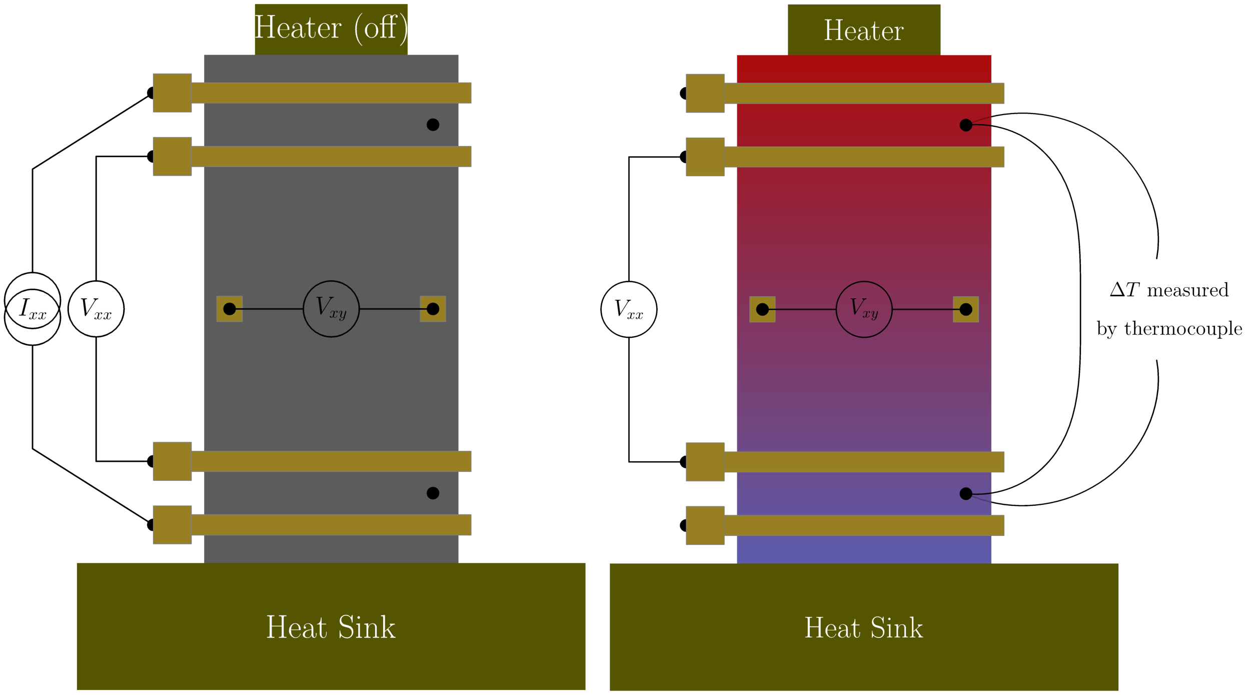


Figure S7: Explanation of which components of the combined experimental setup are used for each measurement. Left: for transport and Hall measurements, a current $I_{xx}$ is run through the sample, and voltage is measured across $V_{xx}$ and $V_{xy}$. For Seebeck and Nernst measurements, a temperature gradient is generated by a heater and heat sink. The temperature gradient is measured through a thermocouple and voltage is measured across $V_{xx}$ and $V_{xy}$.

## Supplementary Note 3: Details of the Tight-Binding Model

To capture the physics of the near-critical Weyl points in $UCo_{1-x}Ru_xAl$, we construct a simple tight binding model on a cubic lattice with a lattice spacing of 1 Å. That is - the nearest neighbor $\langle ij\rangle$ hopping vectors $r_{ij}$ are $\{\pm1,0,0\},\{0,\pm1,0\},\{0,0,\pm1\}$ in units of Å.

The tight binding model used in this work is composed of three orbitals, $a$, $b$, and $c$, with the corresponding creation and annihilation operators $a^\dagger, a$, $b^\dagger, b$, $c^\dagger, c$. The Hamiltonian can be written as

$$\mathcal{H} = \mathcal{H}_0 + \mathcal{H}_{so} + \mathcal{H}_c + \mathcal{H}_{int}$$

where the base tight-binding model, $\mathcal{H}_0$, can be written

$$\mathcal{H}_0 = \sum_i \varepsilon_a a^\dagger_{i\alpha} a_{i\alpha} + \varepsilon_b b^\dagger_{i\alpha} b_{i\alpha} - \sum_{\langle ij\rangle} t_a a^\dagger_{i\alpha} a_{j\alpha} + t_b b^\dagger_{i\alpha} b_{j\alpha} + \sum_{\langle ij\rangle} \frac{\gamma}{2}\left(\hat{z}\cdot\boldsymbol{r}_{ij}\right)\left(a^\dagger_{i\alpha} a_{j\alpha} + b^\dagger_{i\alpha} b_{j\alpha}\right) + h.c. \tag{2}$$

where for simplicity, the onsite energies and hopping energies are set to be equal in magnitude, $\varepsilon_a = -\varepsilon_b = \varepsilon$, $t_a = -t_b = t$. We also have the site indices, $i, j$, bonds $\langle ij\rangle$, and the spin index $\alpha = \uparrow,\downarrow$. The final term above controls the tilting of the Weyl points along the $k_z$ direction, with the critical transition between Type-I and Type-II occurring when $2\gamma = t_a$ The spin orbit term is

$$\mathcal{H}_{so} = \sum_{ij} i\nu_{ij} \boldsymbol{t}_{so}\cdot\boldsymbol{\sigma} \tag{3}$$

where $\nu_{ij} = sgn(\boldsymbol{r}_{ij})$, $\boldsymbol{t}_{so}$ is the the vector of spin orbit coefficients, and $\boldsymbol{\sigma} = \{\sigma_x,\sigma_y,\sigma_z\}$ is the vector of Pauli matrices. This spin orbit coupling term only acts within the space of the $a$ and $b$ orbitals. Together, the first two terms, $\mathcal{H}_0 + \mathcal{H}_{so}$ result in a two band tight-binding model with Weyl points that is similar to models commonly used for WSMs [S5, S3].

In order to faithfully represent the Weyl *metal* nature of the $UCo_{1-x}Ru_xAl$ system (rather than WSM), we introduce an additional band, $c$, that generates a finite density of states at the Weyl energy. Additionally, this band does not have spin-orbit coupling, in order to avoid the creation of additional topological features within the Brillouin zone. This is done through the term

$$\mathcal{H}_c = \sum_i \varepsilon_c c^\dagger_{i\alpha} c_{i\alpha} - \sum_{\langle ij\rangle} t_c c^\dagger_{i\alpha} c_{j\alpha} + h.c \tag{4}$$

where $\varepsilon_c$ and $t_c$ are the corresponding onsite and hopping energies for band $c$. Finally, we introduce a Hubbard interaction term

$$\mathcal{H}_{int} = U\sum_i n_{i\uparrow} n_{i\downarrow} \tag{5}$$

where $n_{i\alpha} = a^\dagger_{i\alpha} a_{i\alpha} + b^\dagger_{i\alpha} b_{i\alpha} + c^\dagger_{i\alpha} c_{i\alpha}$. We treat the interaction term at the mean-field level, that is, we consider fluctuations $\delta n_{i\alpha}$ around the mean value: $n_{i\alpha} = \overline{n_{i\alpha}} + \delta n_{i\alpha}$. Expanding the Hubbard term and neglecting second orders in $\delta n_{i\alpha}$ yields an interaction of the form

$$\begin{aligned}\mathcal{H}_{int} &\approx U\sum_i -\overline{n_{i\uparrow}}\;\overline{n_{i\downarrow}} + \overline{n_{i\uparrow}} n_{i\downarrow} + \overline{n_{i\downarrow}} n_{i\uparrow} \\ &= \frac{U}{4}\left(\overline{n_{i\downarrow}} - \overline{n_{i\uparrow}}\right)^2 - \frac{U}{4}\left(\overline{n_{i\downarrow}} + \overline{n_{i\uparrow}}\right)^2 + \frac{U}{2}\left(\overline{n_{i\downarrow}} + \overline{n_{i\uparrow}}\right)\left(n_{i\downarrow} + n_{i\uparrow}\right) + \frac{U}{2}\left(\overline{n_{i\downarrow}} - \overline{n_{i\uparrow}}\right)\left(n_{i\downarrow} - n_{i\uparrow}\right)\end{aligned} \tag{6}$$

The first three terms either depend on the average values or the total filling, leading to constant shifts, while the last term leads to Stoner-like magnetism splitting the bands. The effective Hamiltonian can thus be written in terms of the magnetization $m = (\overline{n_{i\downarrow}} - \overline{n_{i\uparrow}})$. The full Hamiltonian in $\boldsymbol{k}$-space is:

$$\begin{bmatrix} A_k + \gamma\cos k_z + U\frac{m}{2} & 0 & t^z_{so}\sin k_z & t^x_{so}\sin k_x - it^y_{so}\sin k_y & 0 & 0 \\ 0 & A_k + \gamma\cos k_z - U\frac{m}{2} & t^x_{so}\sin k_x + it^y_{so}\sin k_y & -t^z_{so}\sin k_z & 0 & 0 \\ t^z_{so}\sin k_z & t^x_{so}\sin k_x - it^y_{so}\sin k_y & -A_k + \gamma\cos k_z + U\frac{m}{2} & 0 & 0 & 0 \\ t^x_{so}\sin k_x + it^y_{so}\sin k_y & -t^z_{so}\sin k_z & 0 & -A_k + \gamma\cos k_z - U\frac{m}{2} & 0 & 0 \\ 0 & 0 & 0 & 0 & C_k + U\frac{m}{2} & 0 \\ 0 & 0 & 0 & 0 & 0 & C_k - U\frac{m}{2} \end{bmatrix}$$

$$\begin{aligned} A_k &= \varepsilon - 2t\left(\cos k_x + \cos k_y + \cos k_z\right) \\ C_k &= \varepsilon_c - 2t_c\left(\cos k_x + \cos k_y + \cos k_z\right) \end{aligned} \tag{7}$$

The magnetization $m$ is found self consistently by integrating the density of states $g_\sigma(E)$:

$$m = \int_{-\infty}^{\infty} dE g_\downarrow(E)\theta(E - E_F) - \int_{-\infty}^{\infty} dE g_\uparrow(E)\theta(E - E_F)$$
$$= \int_{-\infty}^{E_F} dE g_\downarrow(E) - \int_{-\infty}^{E_F} dE g_\uparrow(E) \quad (8)$$

In practice, the self consistent solution is obtained as follows. After an initial guess for $m$, the Fermi energy $E_F$ and density of states in each spin channel $g_\sigma(E)$ are computed using tetrahedron integration on a $31 \times 31 \times 31$ $\boldsymbol{k}$-point grid

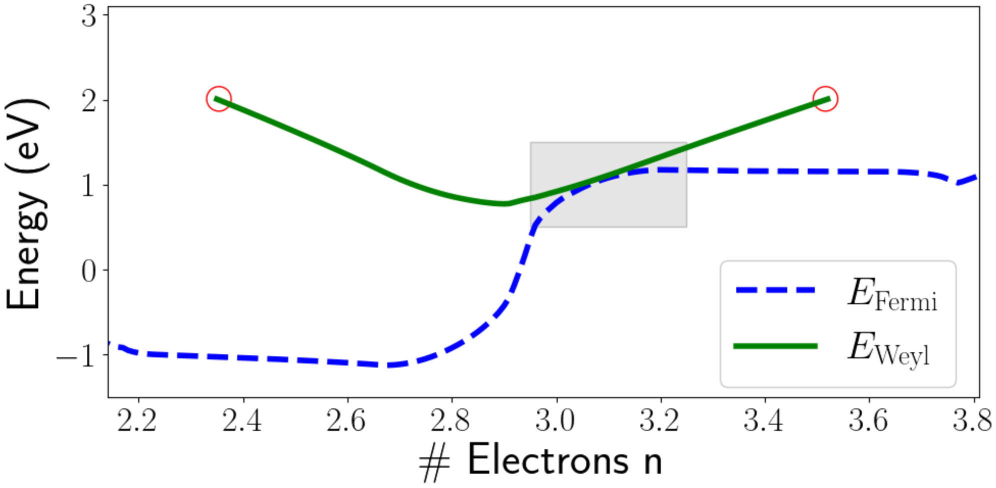


Figure S8: Weyl energy and Fermi energy for alternate model.

The parameters for the model are chosen as follows: $U = 4$ eV, $\varepsilon = 7$ eV, $t = 1$ eV, $t^{\xi}_{so} = \{1, 1, 0\}eV$ and $\gamma = 2t - 10^{-3}$ eV to tilt the Weyl points close to the transition between Type-I and Type-II. In order to mimic the large density of states in $UCo_{1-x}Ru_xAl$, an additional narrow band with $t_c = 0.3$ eV was introduced. When this band is placed at $\varepsilon_c = -1.69$ eV, at a filling $n = 3.088$ the Weyl crossings have a minimal energy of 27 meV above the Fermi level, in line with prior DFT simulations [S2]. The Weyl points in the model have a larger separation than in the DFT calculation.

Figure S8 shows the behavior of the Fermi level and the energy of the Weyl points as a function of the electron filling. As the filling decreases, the Weyl points first appear at $n = 3.516$, and move to lower energy as the band splitting increases with increasing magnetization of the system. Concurrently, the Fermi level remains relatively constant, becoming pinned to the flat band hosting the Weyls between $n = 3.2$ and $n = 3.0$, before rapidly dropping due to a band becoming fully unoccupied as the system passes through $n = 3.0$ half filling. With further decreasing filling from $n = 3.0$ to $n = 2.0$, the magnetization of the system decreases, leading to the annihilation of the Weyl points around $n = 2.354$. As we will show below, the tandem motion of the Weyl points and the Fermi energy in the gray region in Fig. S8, followed by the rapid motion of $E_F$ away from the Weyls, fully determines the shape of the AHE and ANE as a function of doping, rather than the Mott relationship between them.

The computed anomalous Hall and anomalous Nernst coefficients for this model are shown in Figure S9. In the plot, $\alpha_{xy}$ and $\sigma_{xy}$ peak simultaneously around a doping of $n = 3.1$, clearly appearing to violate the Mott relation. However, plots of $\alpha_{xy}$ and $\sigma_{xy}$ vs energy at specific dopings show that the relation still holds.

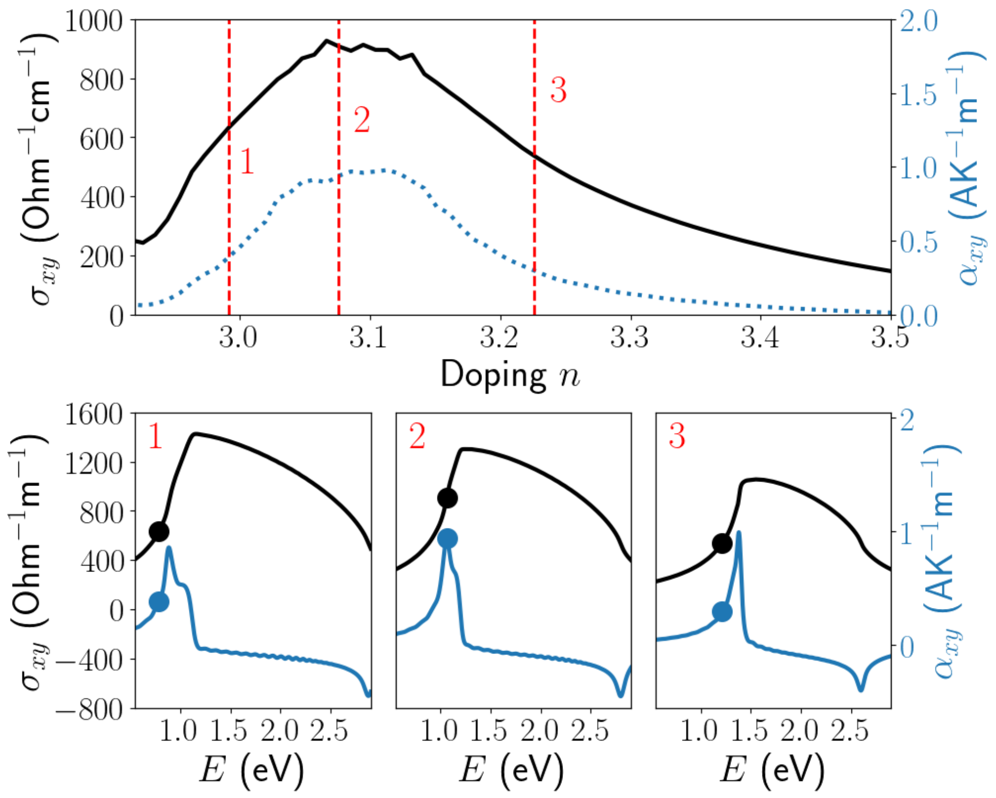


Figure S9

# References


[S1] A. V. Andreev, V. Sechovsky, L. Havela, J. Šebek, M. I. Bartashevich, T. Goto, K. Kamishima, D. A. Andreev, V. S. Gaviko, R. V. Dremov, and I. K. Kozlovskaya. Onset of ferromagnetism between the paramagnets ucoal and urual. *Czechoslovak Journal of Physics*, 46(6):3385–3386, Jun 1996.

[S2] T. Asaba, V. Ivanov, S. M. Thomas, S. Y. Savrasov, J. D. Thompson, E. D. Bauer, and F. Ronning. Colossal anomalous Nernst effect in a correlated noncentrosymmetric kagome ferromagnet. *Science Advances*, 7(13), 2021.

[S3] Jonathan Noky, Johannes Gooth, Claudia Felser, and Yan Sun. Characterization of topological band structures away from the fermi level by the anomalous nernst effect. *Phys. Rev. B*, 98:241106, Dec 2018.

[S4] Jiří Pospíšil, Petr Opletal, Michal Vališka, Yo Tokunaga, Anne Stunault, Yoshinori Haga, Naoyuki Tateiwa, Béatrice Gillon, Fuminori Honda, Tomoo Yamamura, Vojtěch Nižňanský, Etsuji Yamamoto, and Dai Aoki. Properties and collapse of the ferromagnetism in uco1-xruxal studied in single crystals. *Journal of the Physical Society of Japan*, 85(3):034710, 2016.

[S5] Tomá š Rauch, Huong Nguyen Minh, Jürgen Henk, and Ingrid Mertig. Model for ferromagnetic weyl and nodal line semimetals: Topological invariants, surface states, anomalous and spin hall effect. *Phys. Rev. B*, 96:235103, Dec 2017.

[S6] S. Yu. Savrasov and D. Yu. Savrasov. Full-potential linear-muffin-tin-orbital method for calculating total energies and forces. *Phys. Rev. B*, 46:12181–12195, Nov 1992.
